# Supplementary material for: Data Imputation with Iterative Graph Reconstruction
Source: arXiv:2212.02810 source file (2024-04-15)
Supplement: Supplementary file 1 [file appendix.tex]

\appendix
% \twocolumn[{
% \begin{@twocolumnfalse}

\section*{APPENDIX}

\setcounter{table}{0}   %从0开始编号，显示出来表会A1开始编号
\setcounter{figure}{0}

\subsection{MAR and MNAR}
The missing mechanisms are traditionally divided into three categories according to the data distribution: missing completely at random (MCAR), missing at random (MAR), and missing not at random (MNAR)~\cite{little1987statistical}.
In MCAR, the missing of a value is completely random and does not depend on any other values. In MAR, the missing of a value is only correlated with other observed values while in MNAR, the missing is related to both missing values and observed values.

In this section, we introduce the implementation of MAR and MNAR mechanisms and provide additional experiments based on MAR and MNAR mechanisms.

\subsubsection{Experiments Settings.}
In MAR setting, for each dataset, we sample a fixed subset of features which would be introduced missing values and the remaining of the features would have no missing value. 
Then the missingness would be masked in the fixed subset of features according to the logistic masking model with random weights which takes the features have no missing values as input and outputs a binary mask matrix. 

In MNAR setting, for each dataset, we also sample a fixed subset of features which would have missing values according to the logistic masking model with random weights. While this logistic masking model takes the remaining features as input and outputs the binary mask matrix. Finally, the remaining features would be masked by MCAR mechanism.

\begin{table*}[htb]
 \centering
  \caption{Comparisons of average(*10) and variance of MAE values for missing data imputation on eight datasets with 30\% and 70\% missing ratio of 50\% features with MAR. Results have been enlarged by 10 times for better display effects}
%   \vspace{-0.1in}
    \resizebox{1.0\textwidth}{!}{
    \begin{tabular}{l|cc|cc|cc|cc|cc|cc|cc|cc|}
    \toprule
    \textbf{Models} & \multicolumn{2}{c|}{\textbf{Concrete}} & \multicolumn{2}{c|}{\textbf{Housing}} & \multicolumn{2}{c|}{\textbf{Wine}} & \multicolumn{2}{c|}{\textbf{Heart}} & \multicolumn{2}{c|}{\textbf{DOW30}} & \multicolumn{2}{c|}{\textbf{E-commerce}} & \multicolumn{2}{c|}{\textbf{Diabetes}} & \multicolumn{2}{c|}{\textbf{Yacht}} \\
    \textbf{Ratio} & 30\% & 70\% & 30\% & 70\% & 30\% & 70\% & 30\% & 70\% & 30\% & 70\% & 30\% & 70\% & 30\% & 70\% & 30\% & 70\% \\
    \midrule
    Mean & 1.72 & 1.73 & 1.98 & 1.85 & 1.04 & 1.00 & 2.37 & 2.36 & 1.49 & 1.49 & 2.68 & 2.69 & 4.30 & 4.41 & 2.00 & 2.13 \\
    KNN & 0.61 & 0.98 & 0.71 & 0.82 & \textbf{0.60} & 0.76 & \textbf{0.40} & \textbf{1.23} & \textbf{0.16} & \textbf{0.21} & 2.79 & 2.84 & \textbf{1.29} & \textbf{2.11} & 1.67 & 1.86 \\
    MICE & 1.08 & 1.38 & 1.07 & 1.19 & 0.73 & 0.80 & 2.01 & 2.18 & 0.60 & 0.69 & 2.58 & 2.69 & 3.00 & 3.50 & 1.44 & 1.77 \\
    SVD & 2.21 & 2.51 & 1.49 & 1.84 & 1.30 & 1.37 & 2.51 & 2.95 & 1.03 & 1.19 & 2.85 & 2.92 & 3.44 & 3.79 & 2.54 & 2.74 \\
    Spectral & 1.80 & 2.36 & 1.37 & 1.84 & 0.91 & 1.37 & 2.31 & 2.93 & 0.74 & 1.36 & 2.97 & 3.28 & 4.00 & 4.94 & 2.09 & 2.82 \\
    GAIN & 1.39 & 1.81 & 1.27 & 1.44 & 0.89 & 0.88 & 2.16 & 2.31 & 0.81 & 0.92 & 2.62 & 2.38 & 3.36 & 3.65 & 12.17 & 7.41 \\
    OT & 1.09 & 1.54 & 0.86 & 1.15 & 0.77 & 0.86 & 1.84 & 2.09 & 0.43 & 0.68 & 2.56 & 2.51 & 2.51 & 3.29 & 1.68 & 2.53 \\
    Miracle & 0.97 & 1.46 & 1.29 & 1.71 & 0.78 & 0.85 & 1.98 & 2.53 & 1.70 & 3.86 & 2.40 & 2.75 & 3.13 & 3.29 & 1.90 & 2.53 \\
    GRAPE & 0.65 & 0.98 & 0.71 & 0.84 & 0.64 & 0.71 & 1.35 & 1.81 & 0.19 & 2.26 & 2.56 & 2.82 & 1.98 & 2.75 & 1.41 & 1.84 \\
    IGRM & \textbf{0.60} & \textbf{0.81} & \textbf{0.59} & \textbf{0.75} & 0.61 & \textbf{0.68} & 1.28 & 1.72 & 0.18 & \textbf{0.21} & \textbf{2.31} & \textbf{2.34} & 1.89 & 2.55 & \textbf{0.66} & \textbf{1.17} \\
    \bottomrule
    \end{tabular}%
    }
  \label{tab:imputationwithbaselineMAR}%
%   \vspace{-0.1in}
\end{table*}%

\begin{table*}[htb]
 \centering
  \caption{Comparisons of average(*10) and variance of MAE values for missing data imputation on eight datasets with 30\% and 70\% missing ratio of 50\% features with MNAR. Results have been enlarged by 10 times for better display effects}
%   \vspace{-0.1in}
    \resizebox{1.0\textwidth}{!}{
    \begin{tabular}{l|cc|cc|cc|cc|cc|cc|cc|cc|}
    \toprule
    \textbf{Models} & \multicolumn{2}{c|}{\textbf{Concrete}} & \multicolumn{2}{c|}{\textbf{Housing}} & \multicolumn{2}{c|}{\textbf{Wine}} & \multicolumn{2}{c|}{\textbf{Heart}} & \multicolumn{2}{c|}{\textbf{DOW30}} & \multicolumn{2}{c|}{\textbf{E-commerce}} & \multicolumn{2}{c|}{\textbf{Diabetes}} & \multicolumn{2}{c|}{\textbf{Yacht}} \\
    \textbf{Ratio} & 30\% & 70\% & 30\% & 70\% & 30\% & 70\% & 30\% & 70\% & 30\% & 70\% & 30\% & 70\% & 30\% & 70\% & 30\% & 70\% \\
    \midrule
    Mean & 1.84 & 1.84 & 1.94 & 1.87 & 1.02 & 1.00 & 2.34 & 2.34 & 1.57 & 1.58 & 2.51 & 2.51 & 4.38 & 4.44 & 2.11 & 2.20 \\
    KNN & 1.40 & 1.81 & 1.21 & 1.68 & 1.03 & 1.17 & \textbf{1.39} & 2.41 & 0.50 & 1.20 & 2.88 & 2.88 & 2.61 & 4.27 & 1.99 & 2.87 \\
    MICE & 1.37 & 1.78 & 1.23 & 1.66 & 0.80 & 0.94 & 2.08 & 2.27 & 0.61 & 1.26 & 2.43 & 2.58 & 3.21 & 4.09 & 1.64 & 2.21 \\
    SVD & 2.21 & 2.69 & 1.51 & 2.39 & 1.17 & 1.39 & 2.52 & 3.23 & 1.00 & 1.67 & 2.76 & 3.15 & 3.57 & 4.53 & 2.68 & 3.47 \\
    Spectral & 1.96 & 2.52 & 1.46 & 2.35 & 0.92 & 1.48 & 2.37 & 3.11 & 0.76 & 1.98 & 3.09 & 3.66 & 4.08 & 5.10 & 2.57 & 3.74 \\
    GAIN & 1.68 & 1.86 & 1.62 & 1.80 & 0.93 & 1.48 & 2.37 & 3.11 & 0.76 & 1.98 & 3.09 & 3.66 & 4.08 & 5.10 & 2.57 & 3.74 \\
    OT & 1.16 & 1.76 & 0.90 & 1.34 & 0.77 & 1.01 & 1.81 & \textbf{2.11} & 0.47 & 0.89 & 2.54 & 2.53 & 2.55 & 3.65 & 1.77 & 2.48 \\
    Miracle & 1.30 & 2.07 & 1.38 & 3.01 & 0.74 & 1.71 & 2.05 & 4.32 & 1.11 & 3.35 & 2.44 & 3.47 & 3.37 & 7.73 & 1.95 & 5.66 \\
    GRAPE & 0.92 & 1.64 & 0.77 & 1.25 & 0.67 & 0.90 & 1.58 & 2.13 & \textbf{0.20} & 0.48 & 2.30 & 2.47 & 2.41 & 3.63 & 1.49 & 2.33 \\
    IGRM & \textbf{0.82} & \textbf{1.38} & \textbf{0.67} & \textbf{1.08} & \textbf{0.66} & \textbf{0.87} & 1.54 & \textbf{2.11} & \textbf{0.20} & \textbf{0.29} & \textbf{2.27} & \textbf{2.35} & \textbf{2.25} & \textbf{3.36} & \textbf{1.06} & \textbf{2.00} \\
    \bottomrule
    \end{tabular}%
    }
  \label{tab:imputationwithbaselineMNAR}%
%   \vspace{-0.1in}
\end{table*}%

\subsubsection{Experimental Results.} Table~\ref{tab:imputationwithbaselineMAR} and \ref{tab:imputationwithbaselineMNAR} show the mean of MAE compared with various methods with 30\% and 70\% missing ratios in MAR and MNAR mechanisms, the best result is marked in bold and the results have been enlarged by 10 times.
In MNAR mechanism, IGRM outperforms all baselines in 6 out of 8 datasets and reaches the second best performance in Heart dataset and comparable result in DOW30 dataset. IGRM yields 7.77\% and 12.46\% lower mean MAE than the second-best baseline(GRAPE) in 30\% and 70\% missing respectively.
While in MAR mechanism, IGRM outperforms baselines except KNN in 4 datasets and reaches the best performance in the remaining datasets.
We conjecture this is because, in MAR setting, a subset of features have no missing values, through which KNN can capture similar neighbors accurately.
Results show that IGRM performs well and is robust to difficult missing mechanisms, this is remarkable as IGRM do not attempt to be designed for these missing mechanisms.
In addition, IGRM can also perform well in 70\% missing ratios in both MAR and MNAR mechanisms while the performances of other baselines are usually worse than Mean imputation. This further confirms that the introduction of friend network can effectively alleviate the problem of data sparsity.

\subsection{Additional Evolution of Embeddings}
In this section, to further prove the effectiveness of iterative friend network reconstruction, we show additional cosine similarity deviation evolution during iterative learning at 1st, 1000th, 5000th, 10000th epoch in several datasets. Results illustrated in Fig.~\ref{fig:similarity_iterative_appendix} further prove that embeddings can gradually mitigate the effect of missing data during the model training.

\begin{figure*}[htb]
	\centering 
	\subfigbottomskip=2pt
	\subfigure[Concrete]{
		\includegraphics[width=0.5\columnwidth]{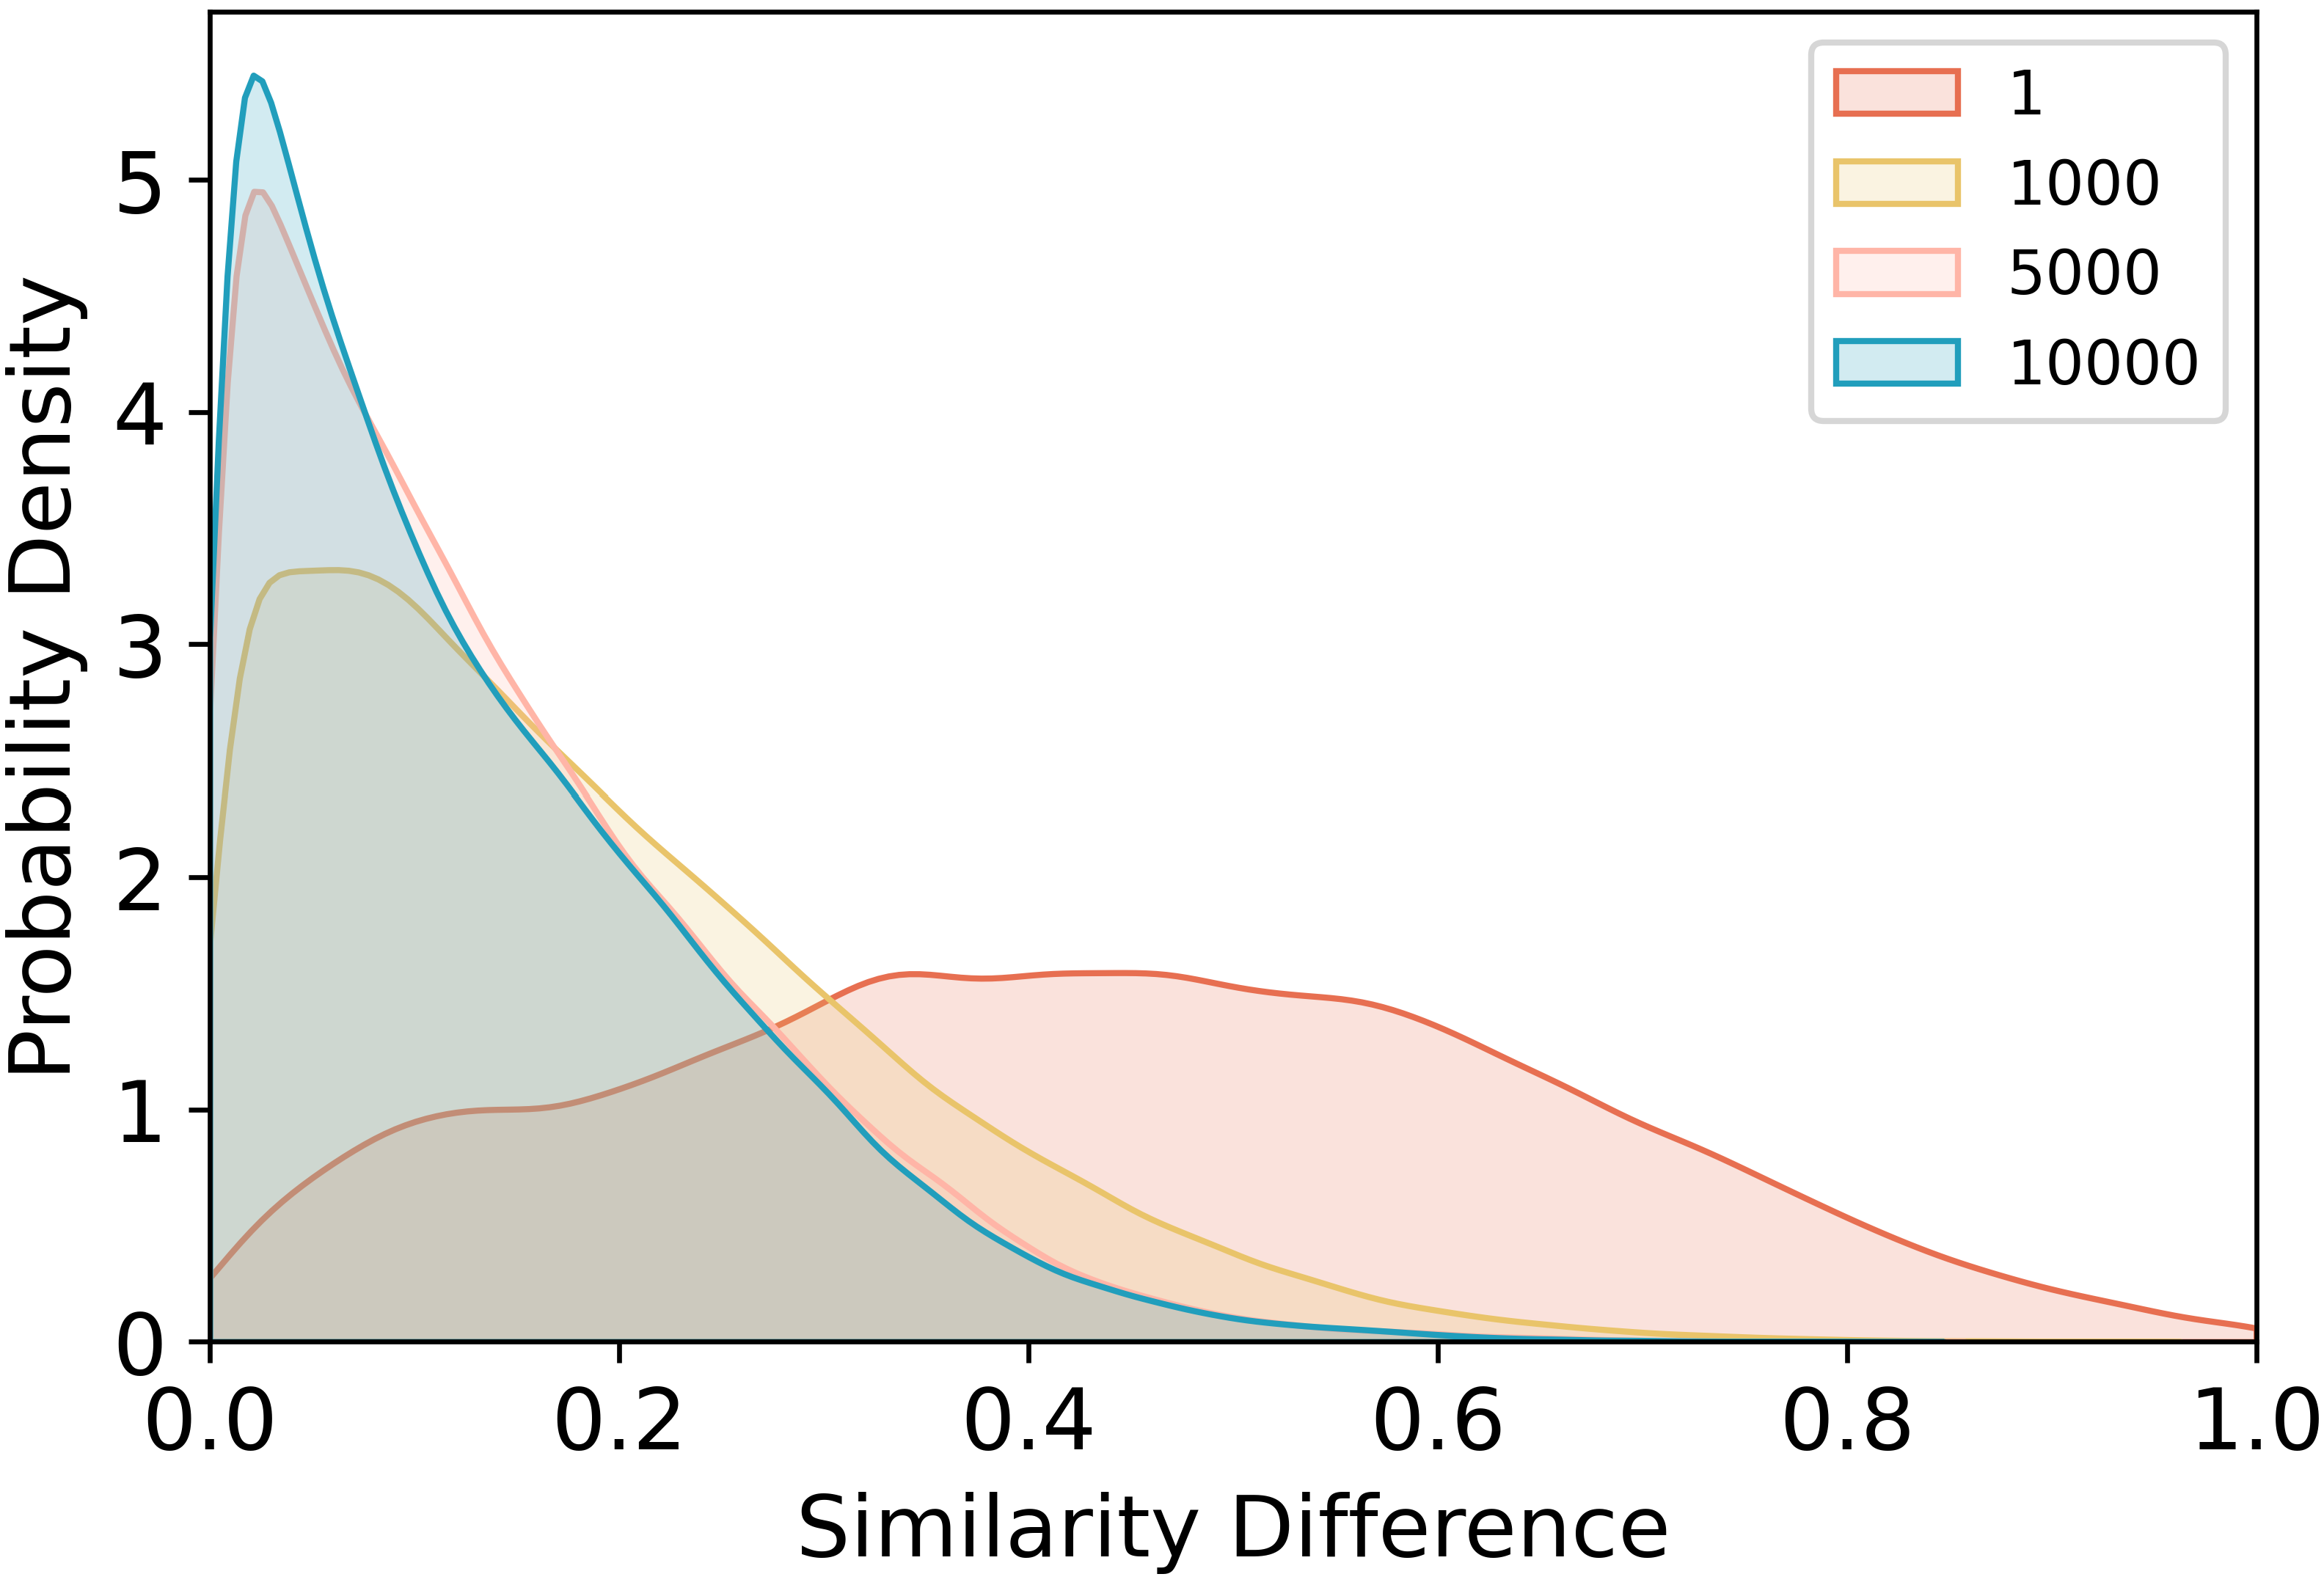}}
    \subfigure[Housing]{
	    \includegraphics[width=0.5\columnwidth]{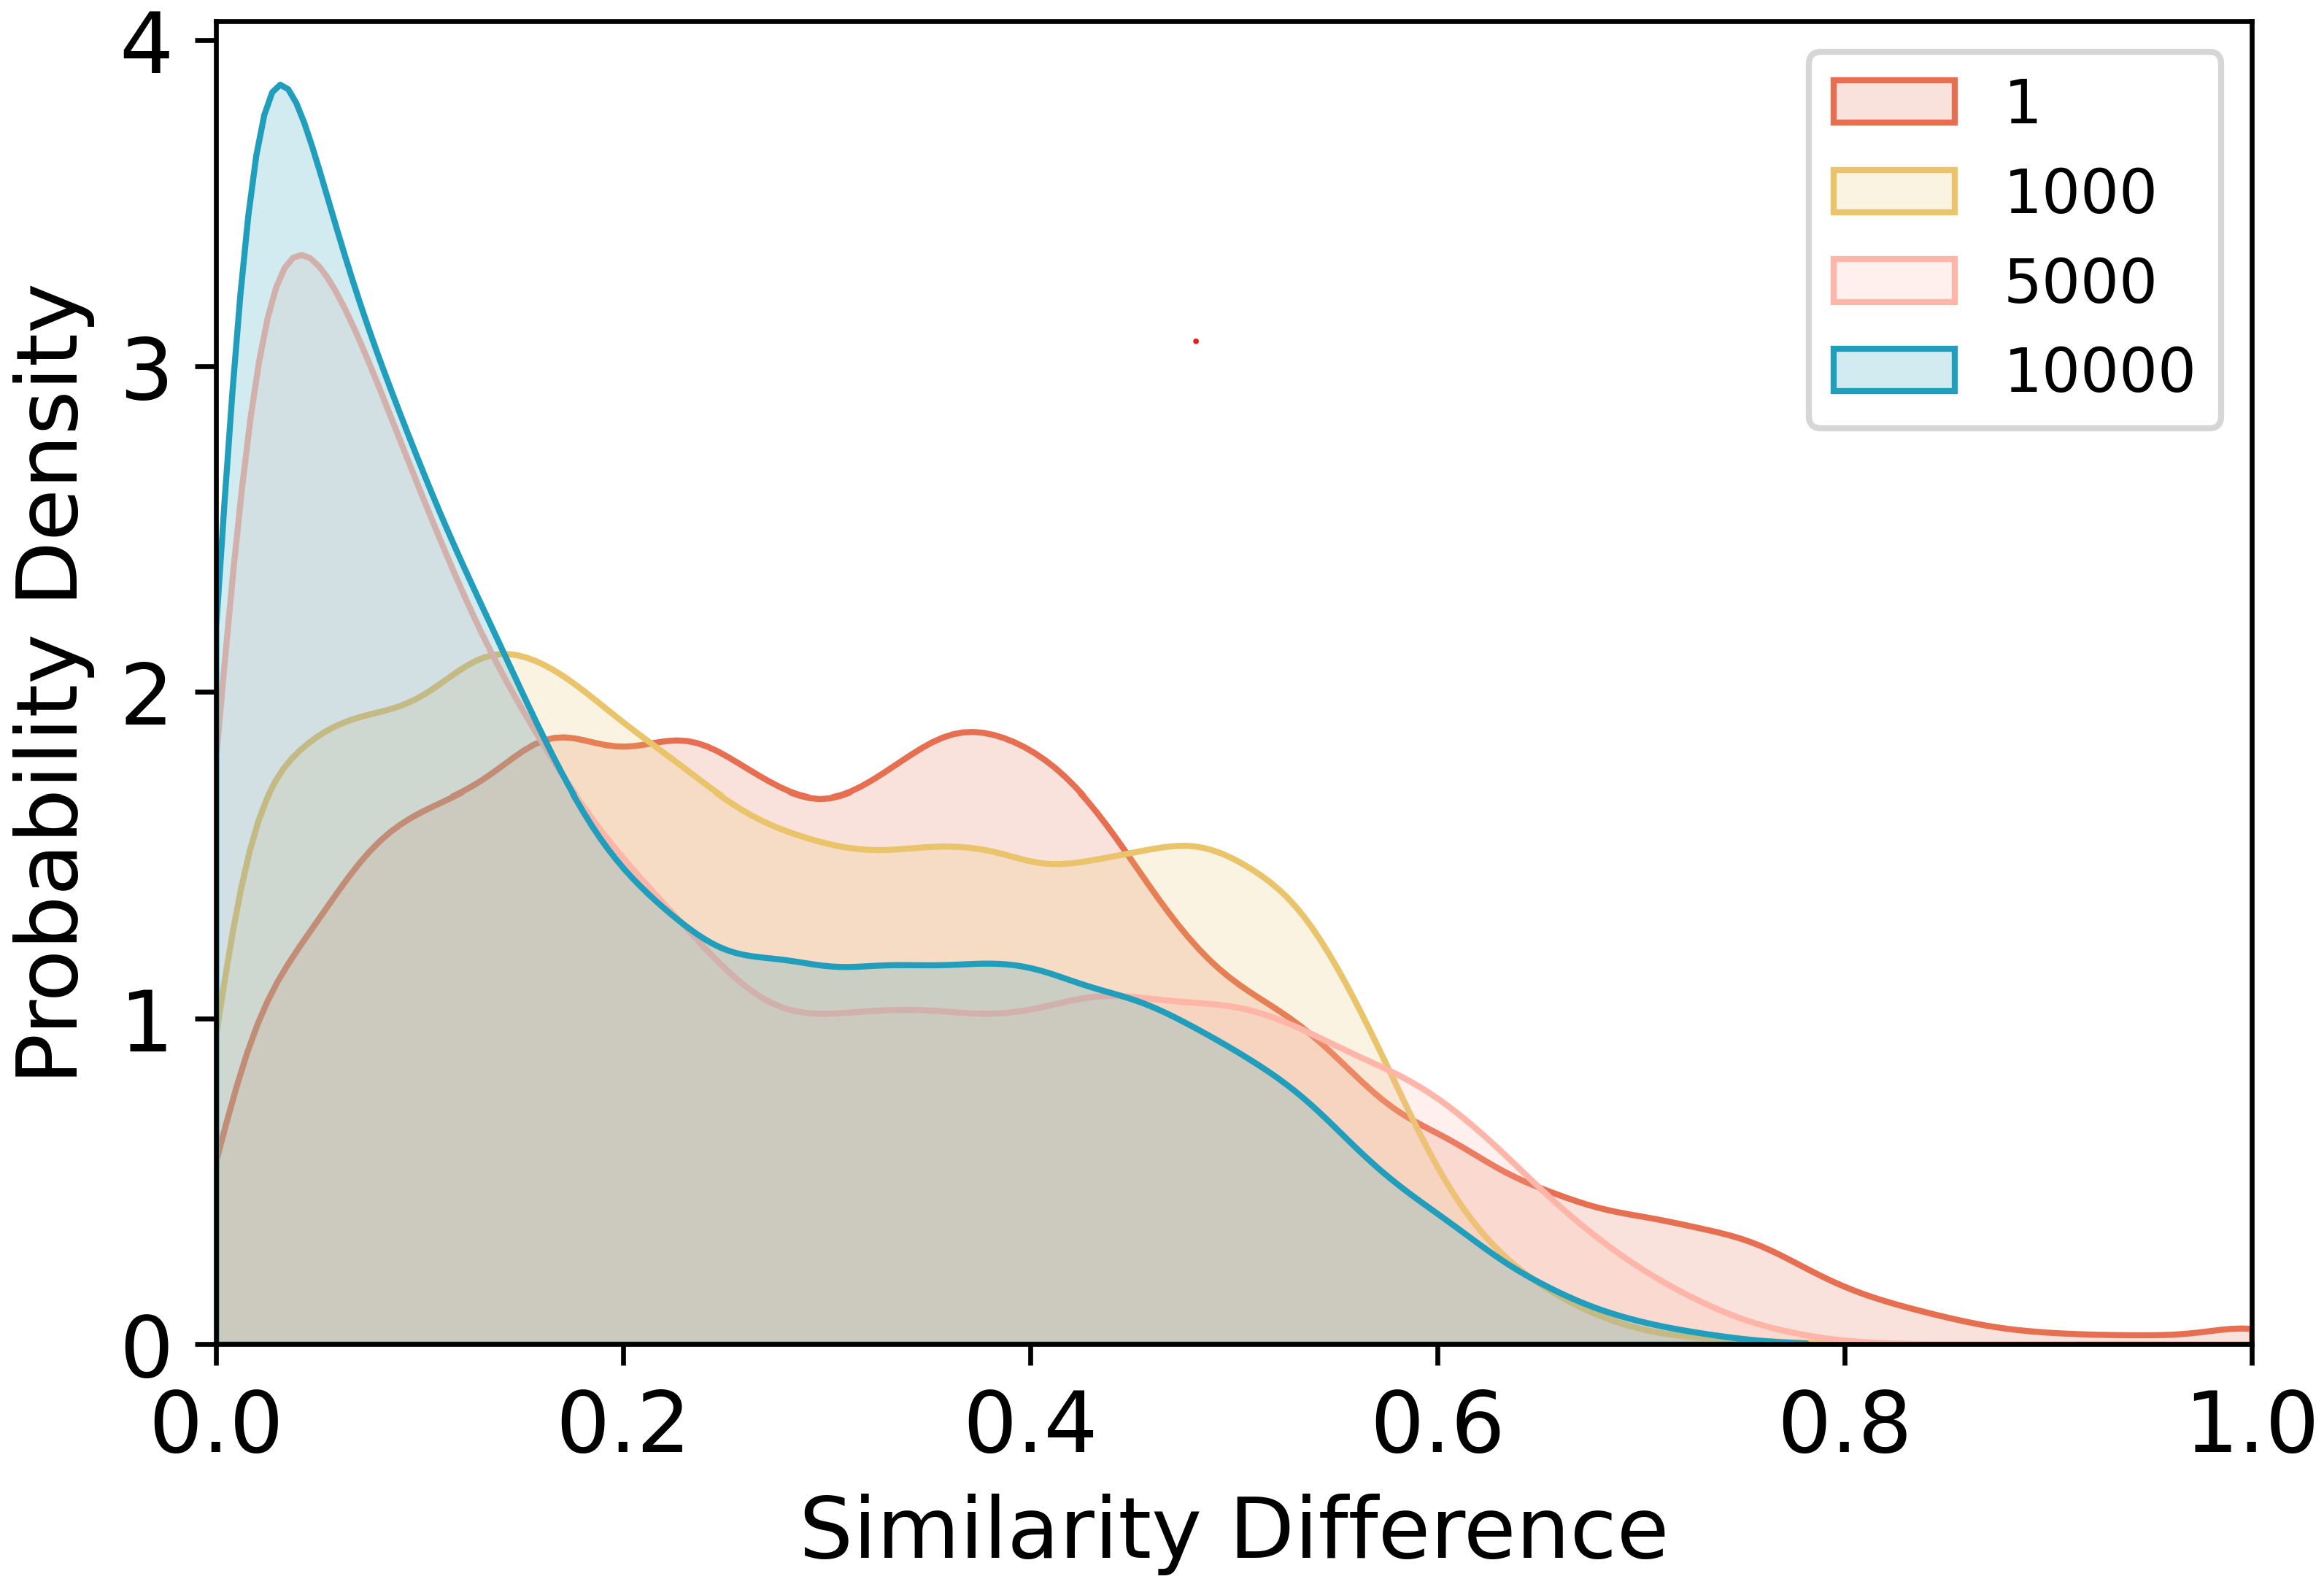}}
	\subfigure[Wine]{
		\includegraphics[width=0.5\columnwidth]{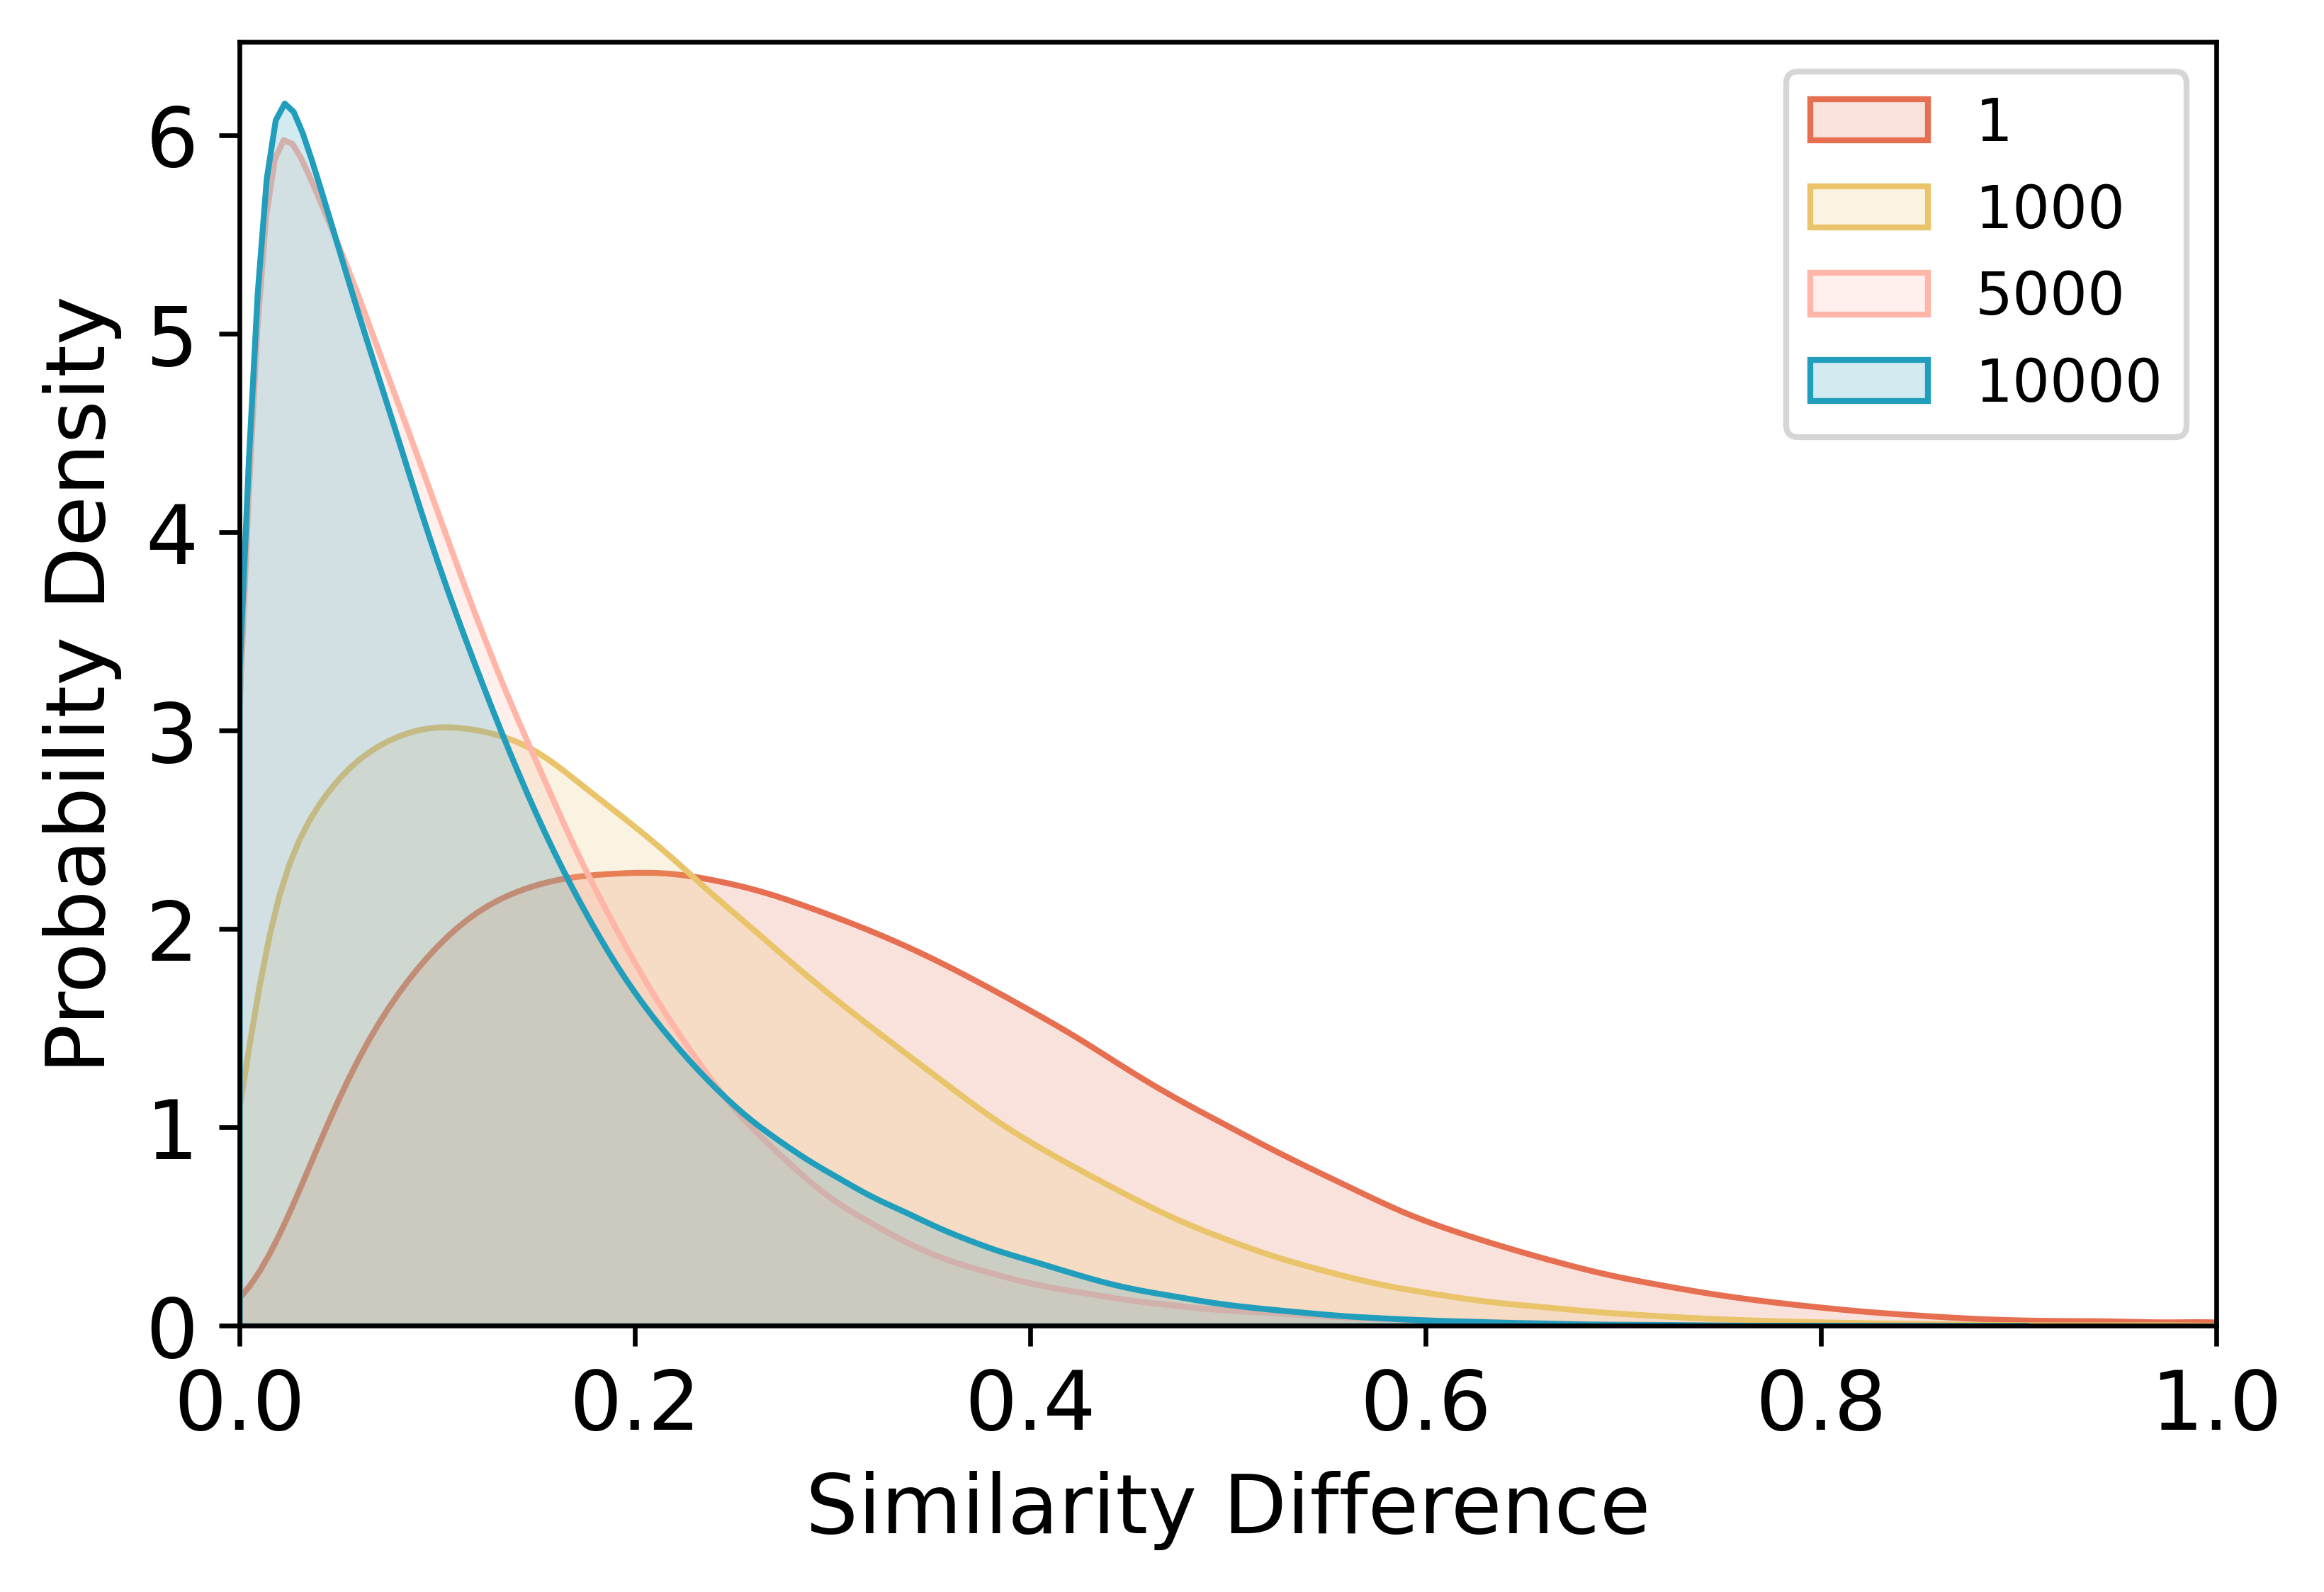}}\\
	\subfigure[Heart]{
		\includegraphics[width=0.5\columnwidth]{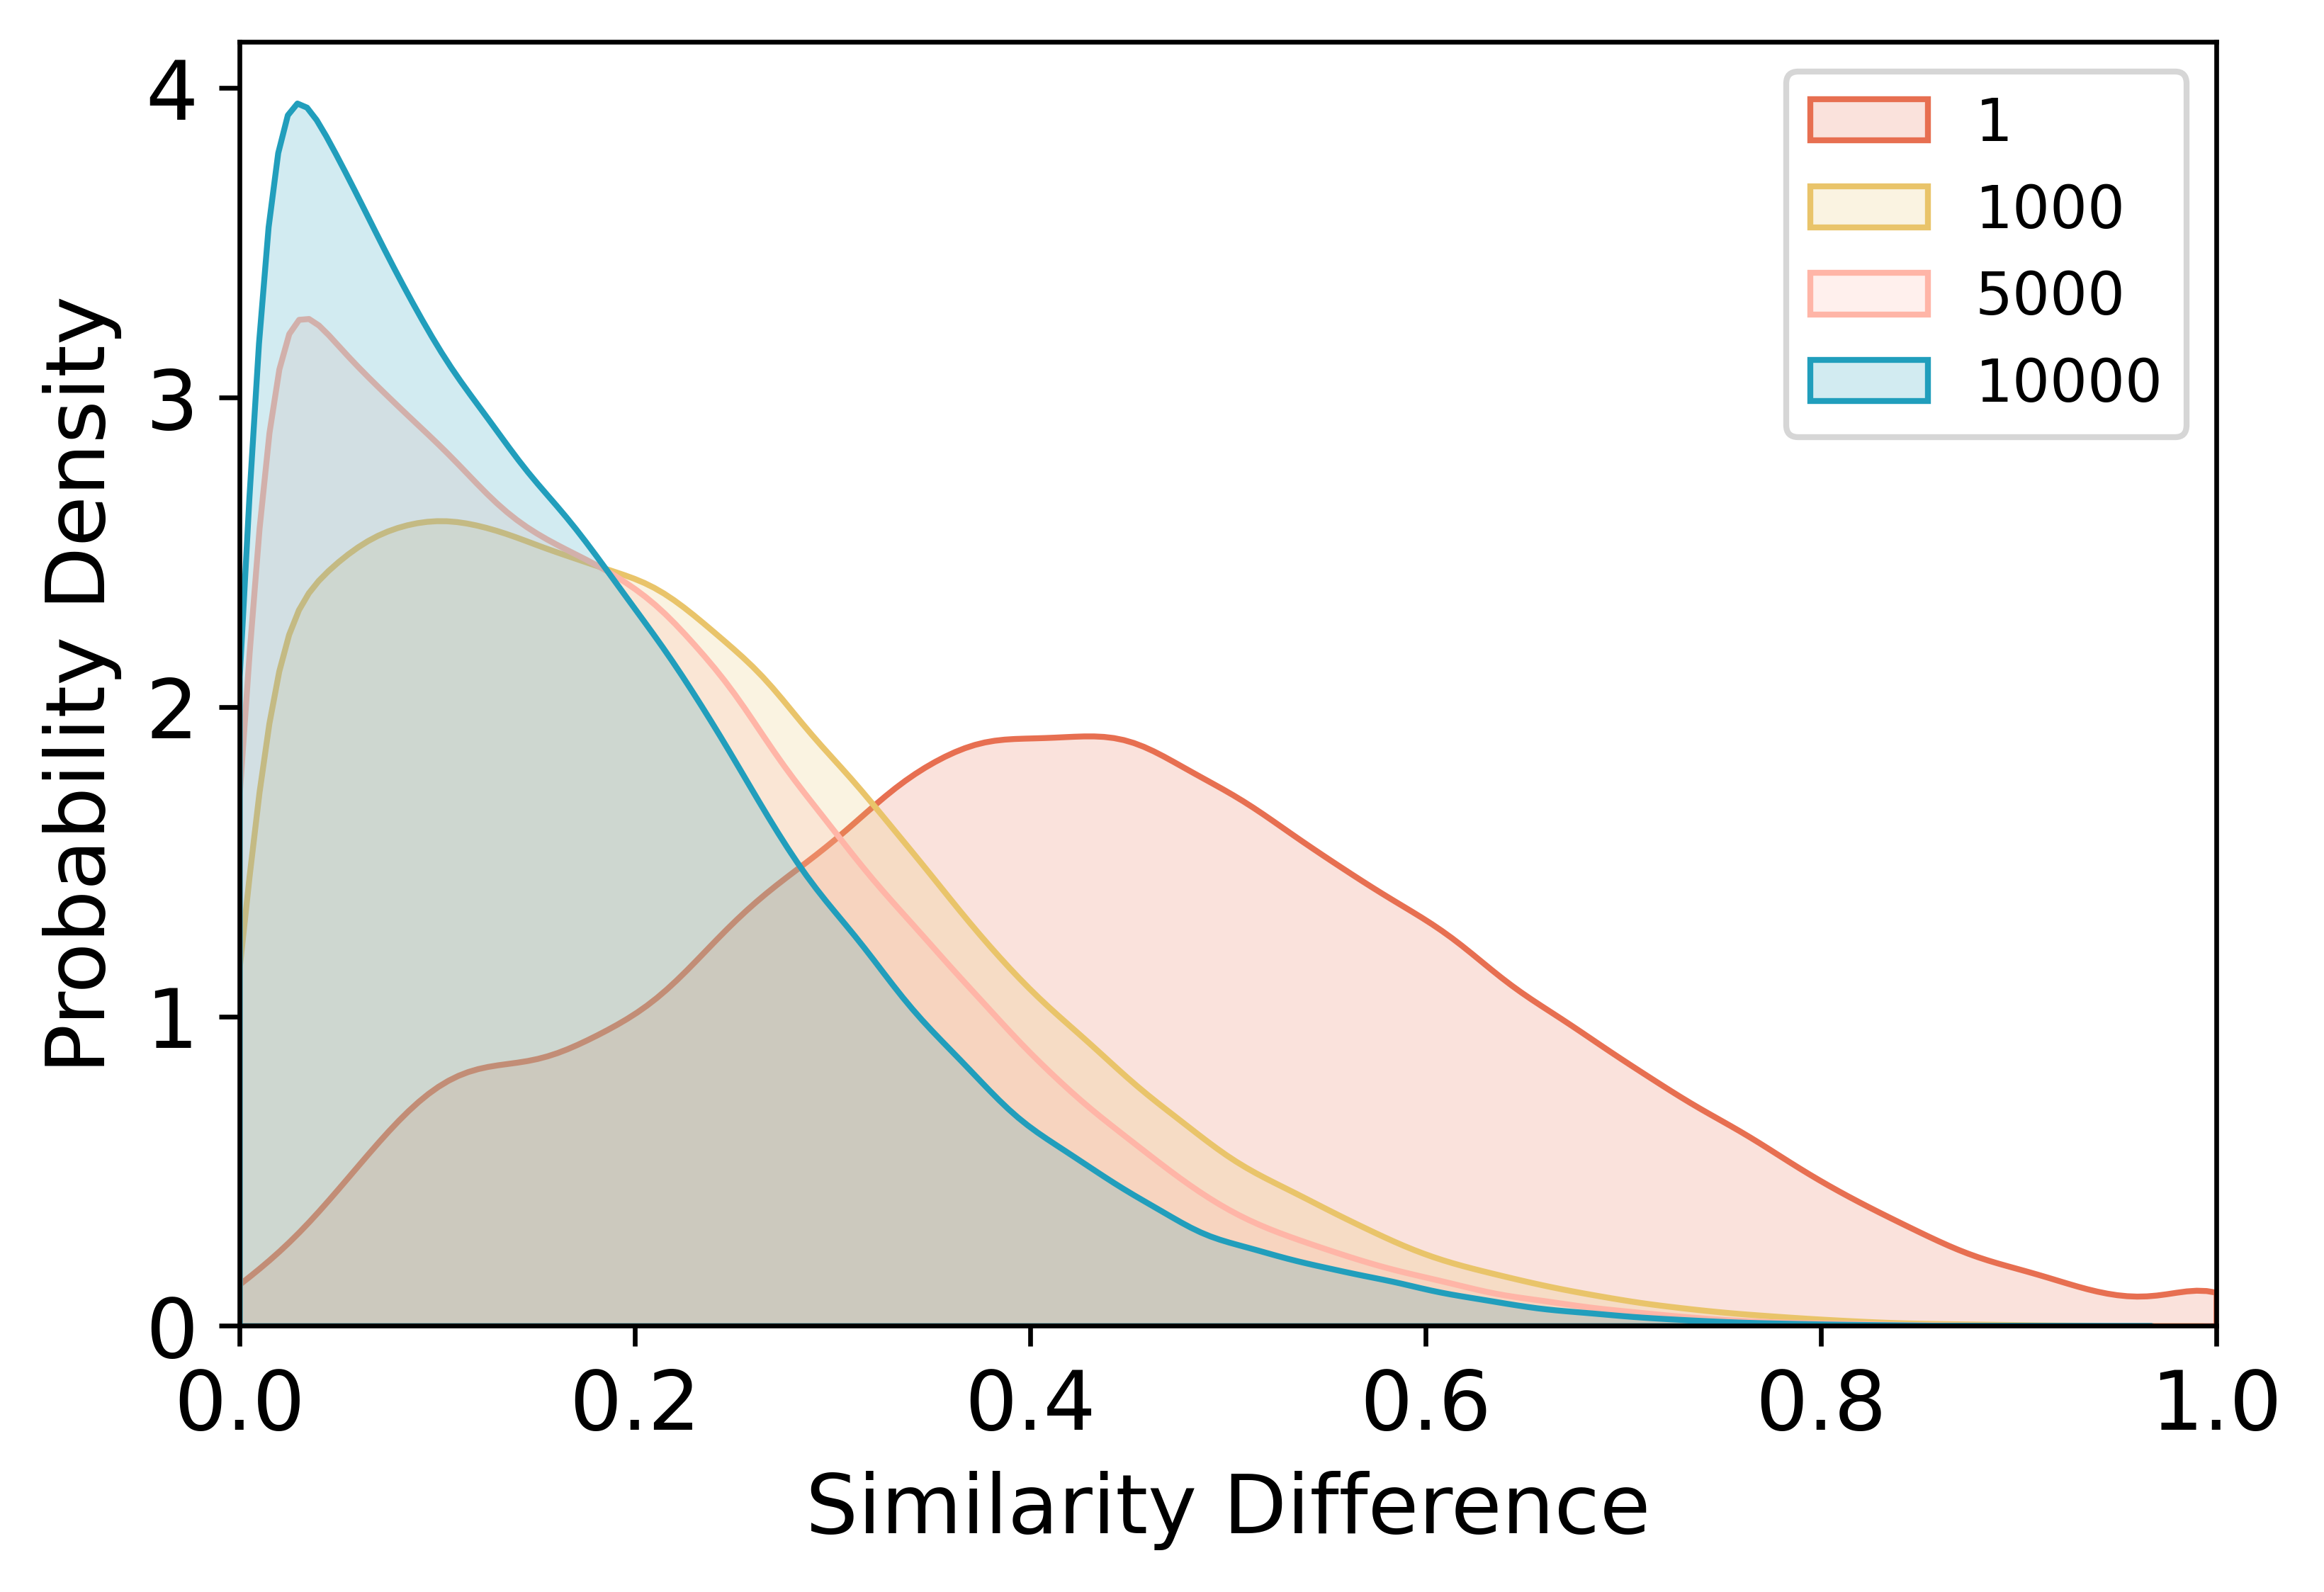}}   
	\subfigure[E-commerce]{
		\includegraphics[width=0.5\columnwidth]{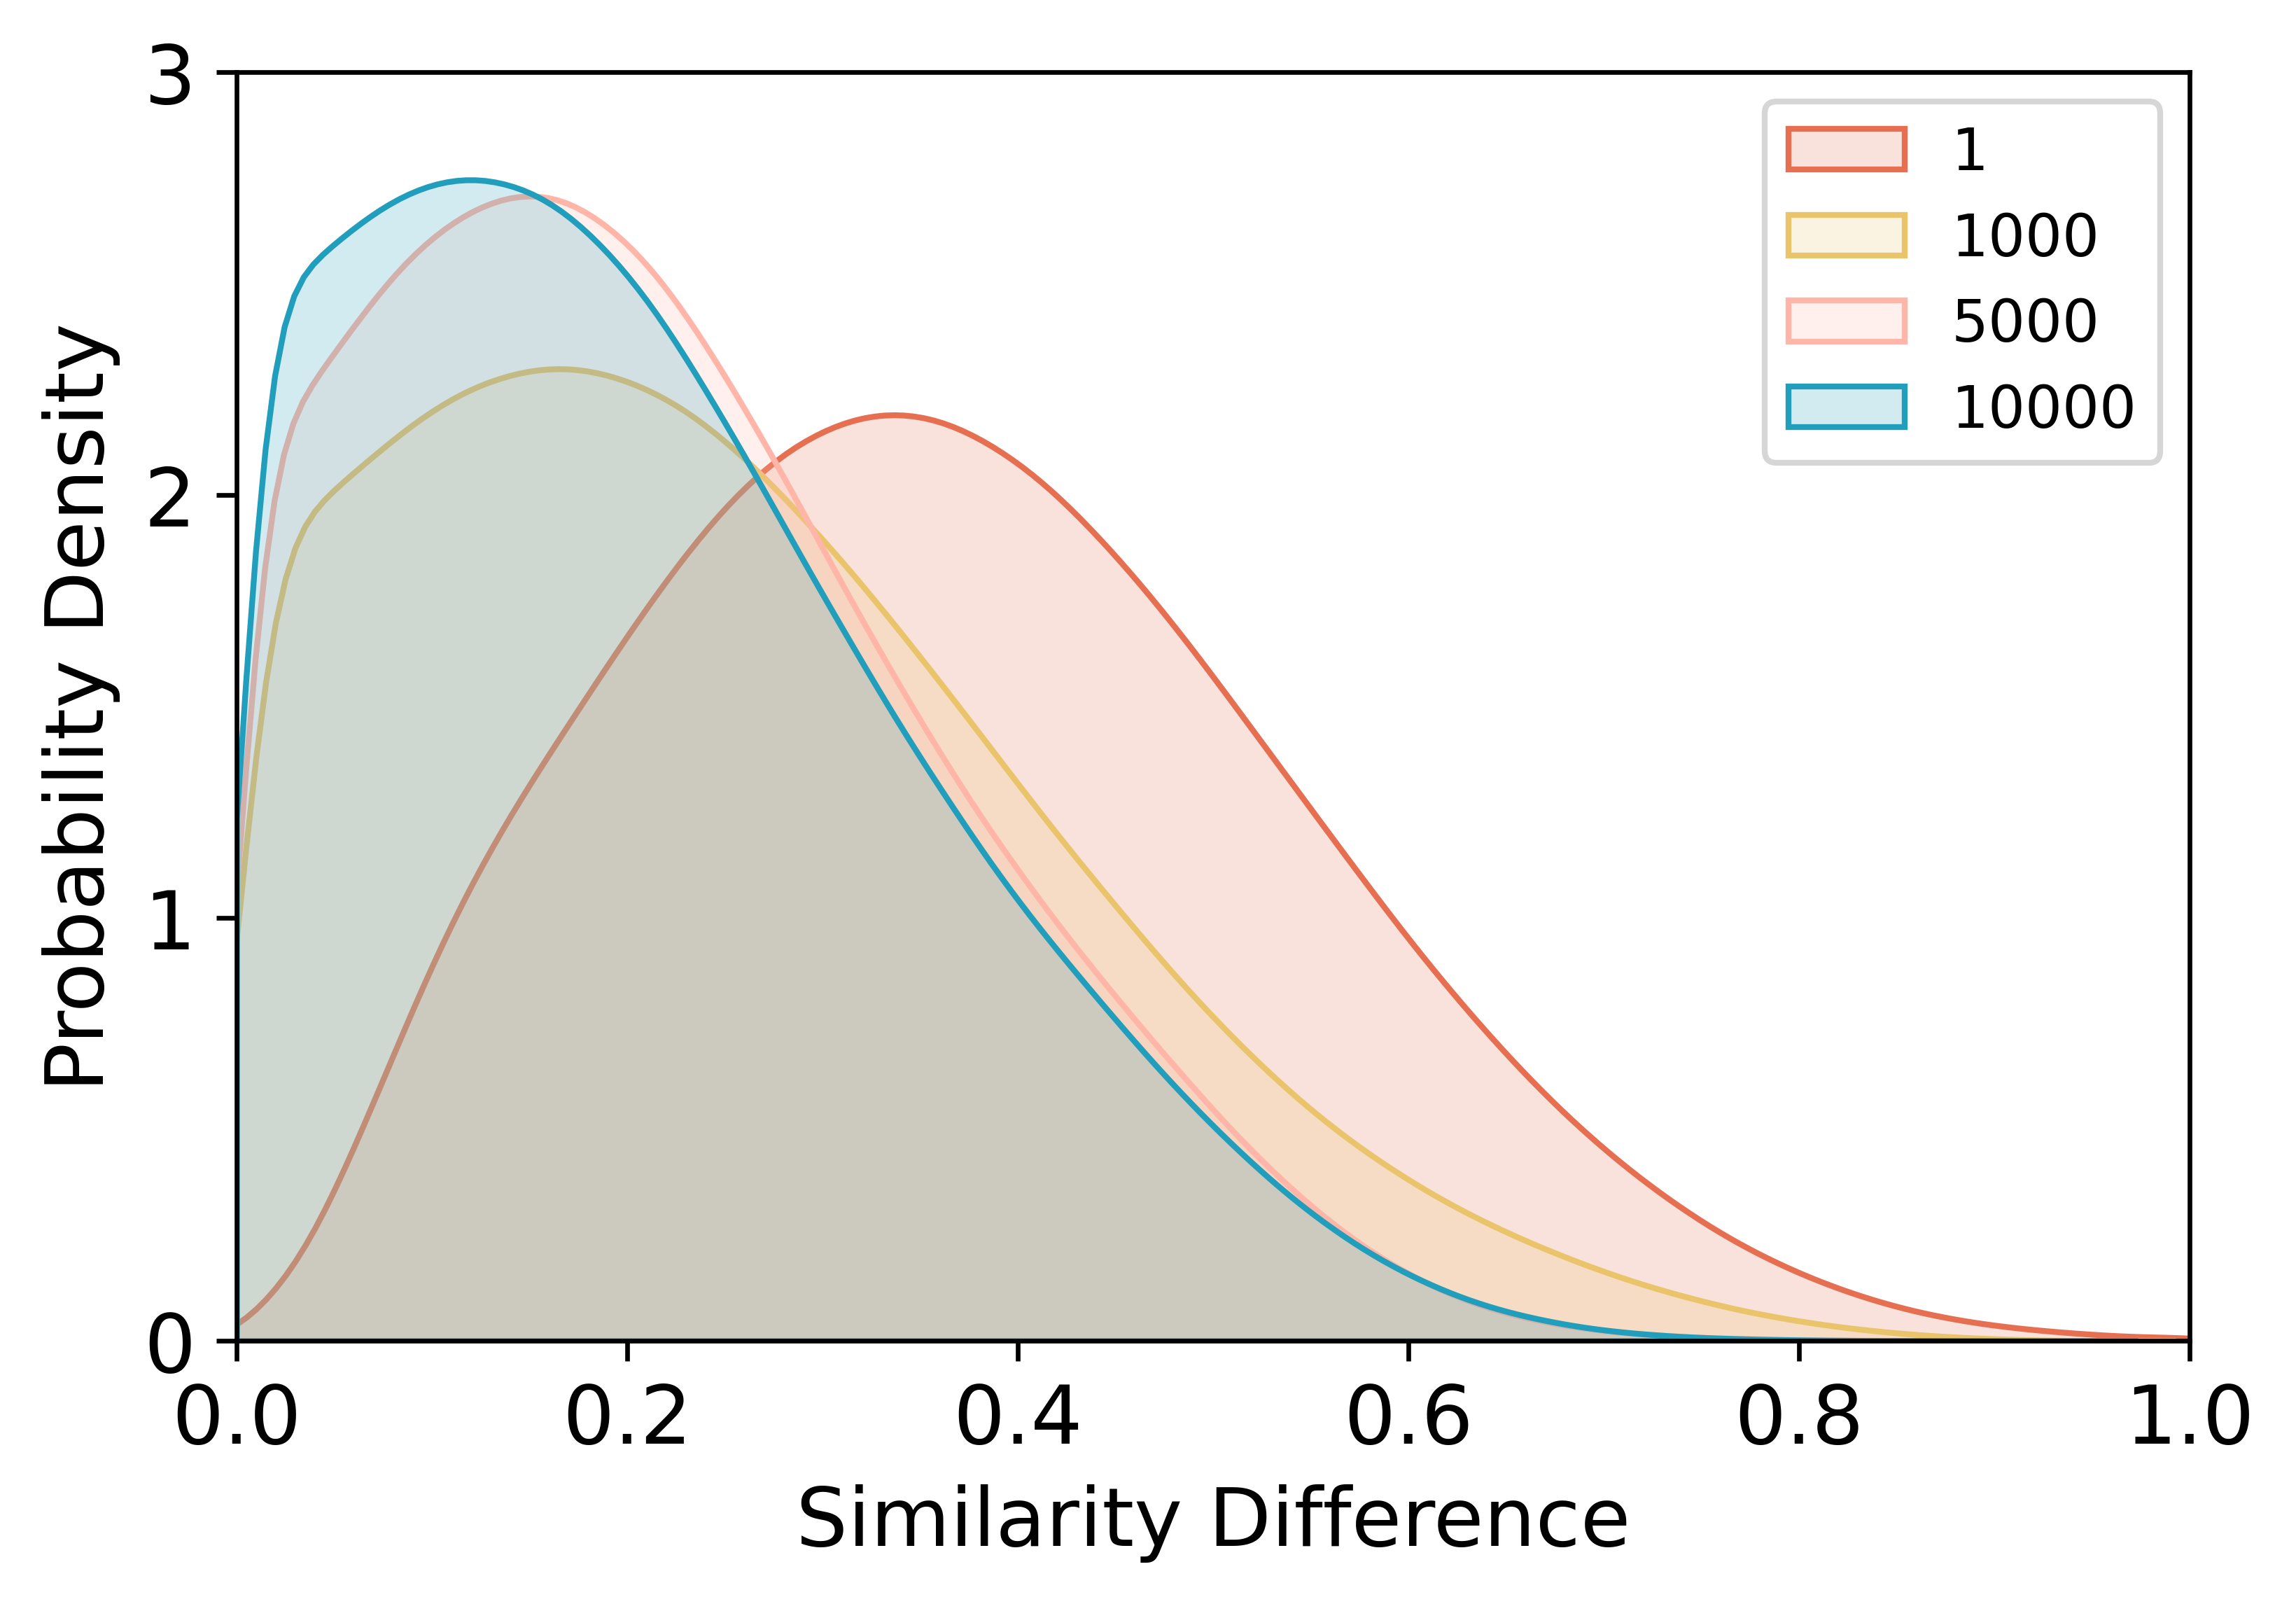}}
	\subfigure[Diabetes]{
		\includegraphics[width=0.5\columnwidth]{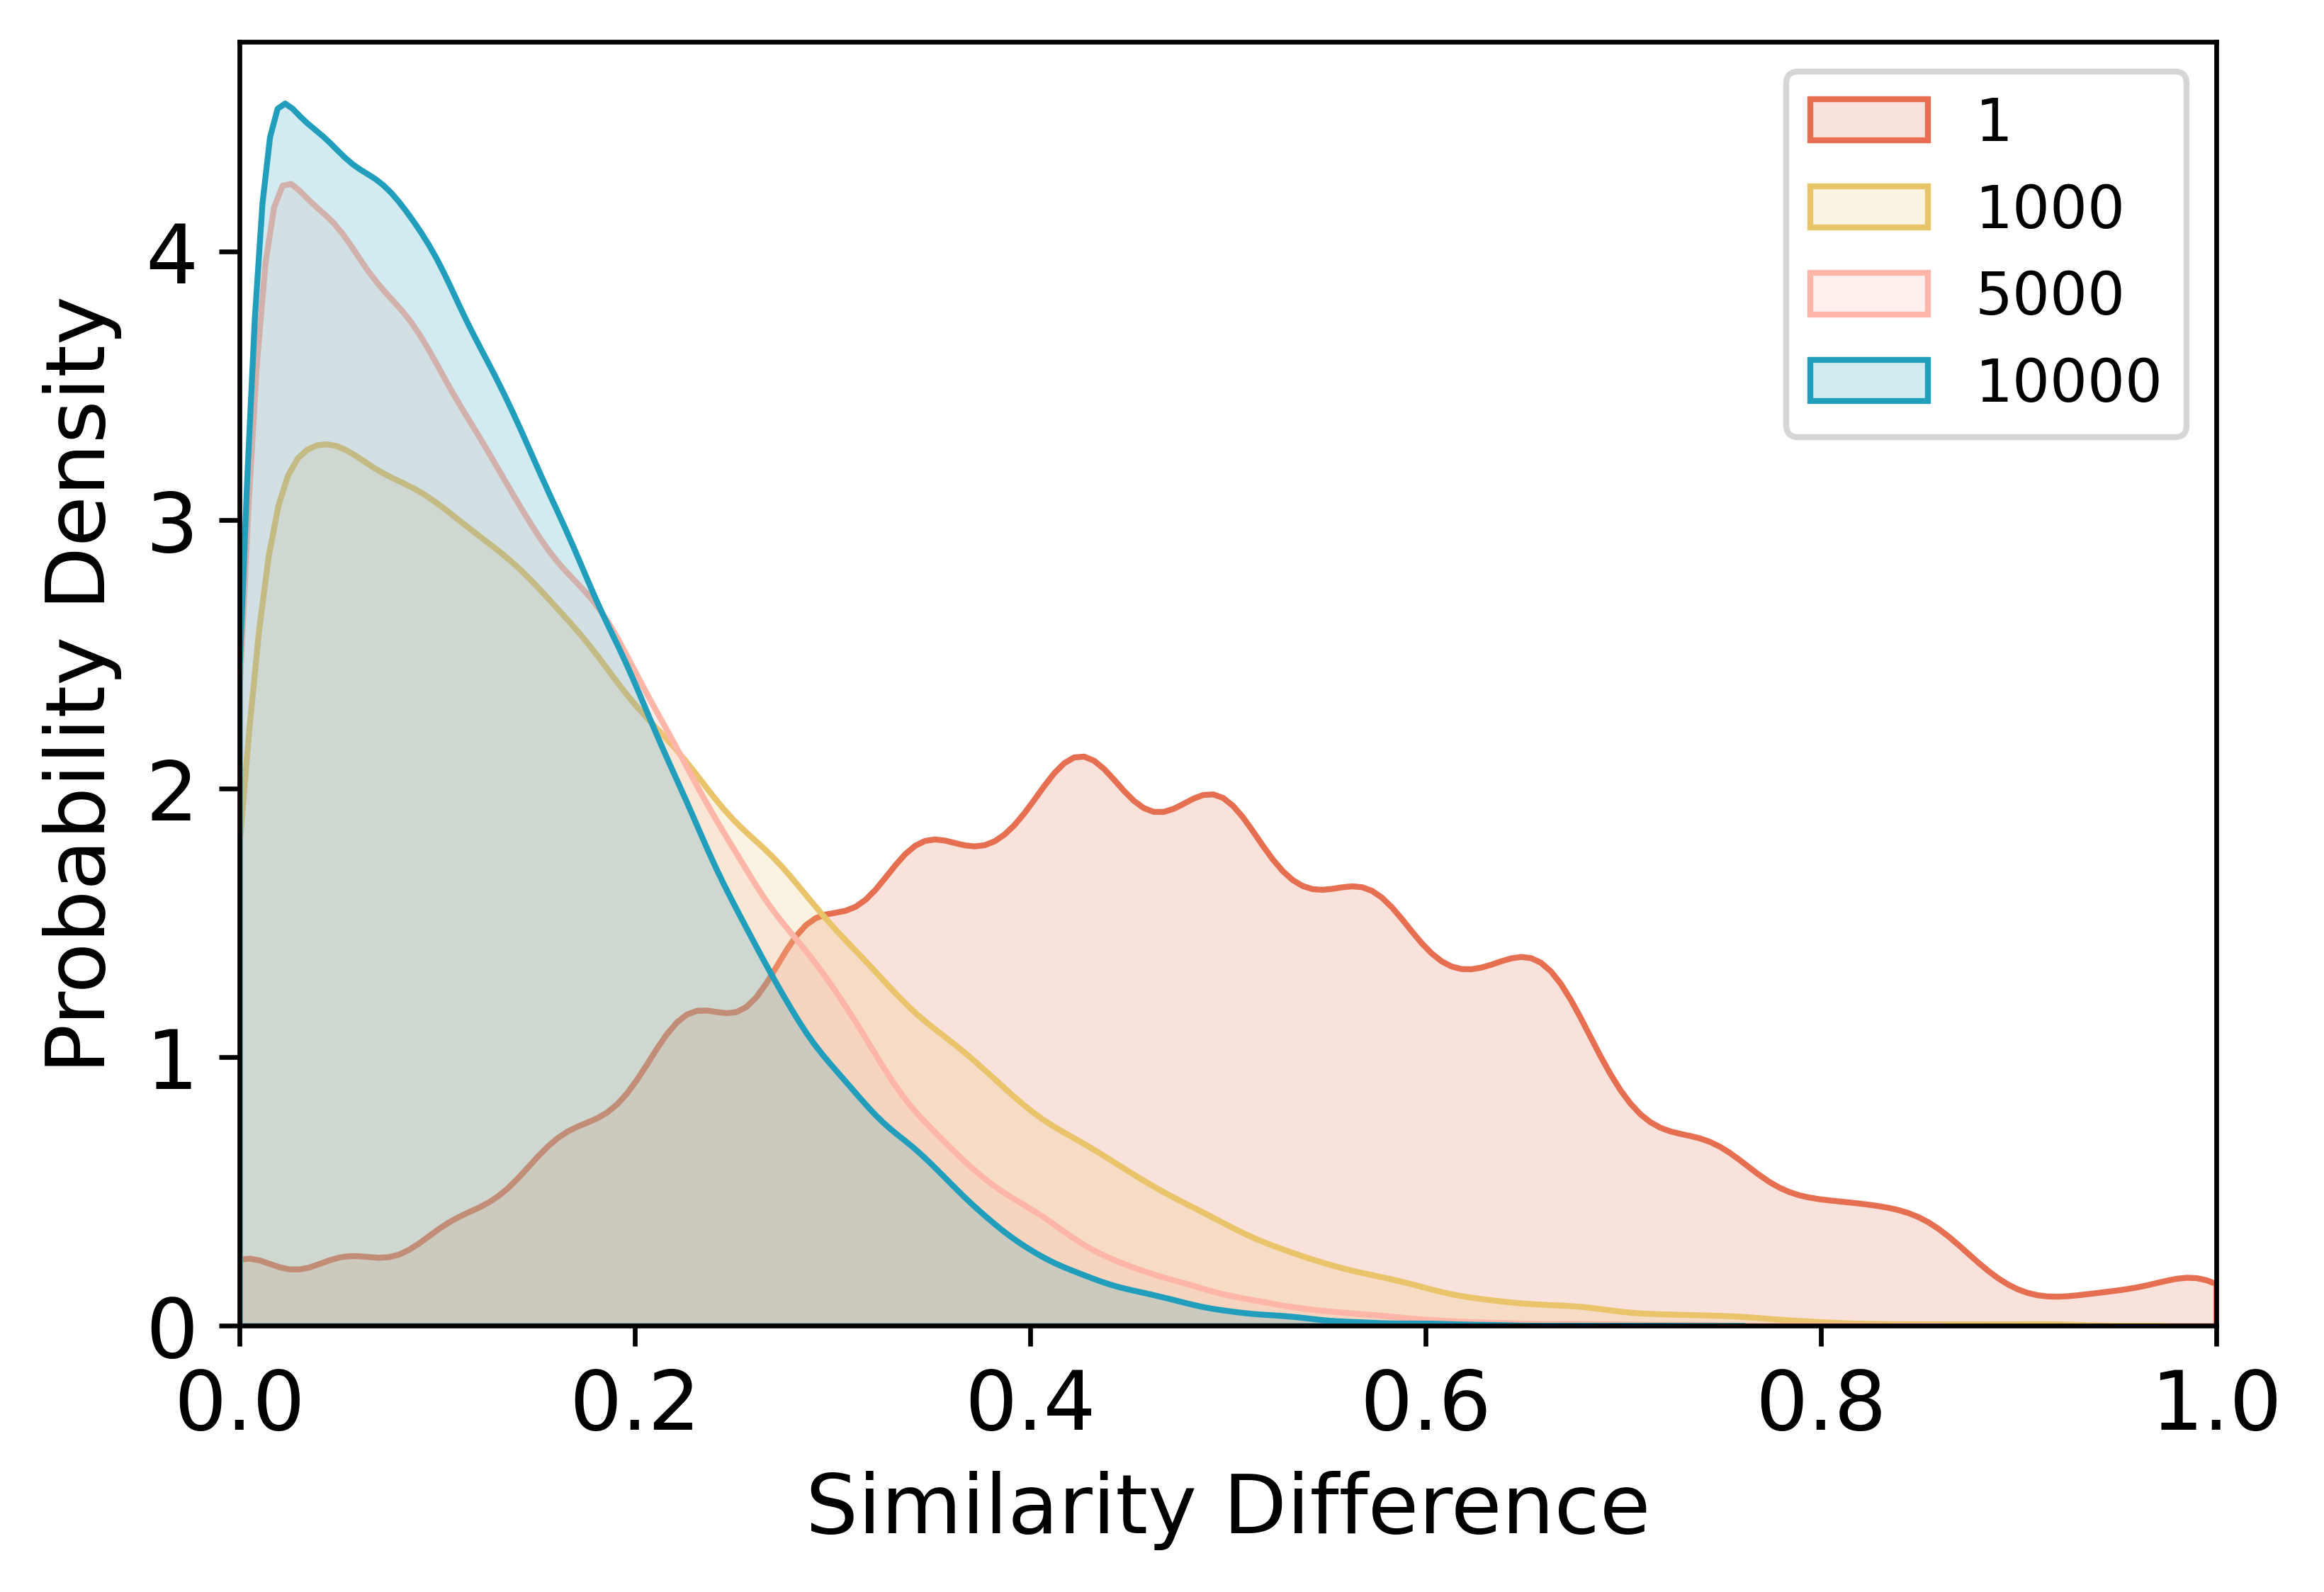}}
    \caption{Similarity deviation distribution. The deviation is the absolute value of the difference between the generated embeddings similarity and the ground-truth similarity.}
	\label{fig:similarity_iterative_appendix}
% 	 \vspace{-0.1in}
\end{figure*}

\subsection{Additional Experiments}
In this section, we provide some additional experiments on more datasets come from UCI~\cite{asuncion2007uci}. The summary statistics of datasets are shown in Table~\ref{tab:datasets_appendix}. The results are shown in Fig.~\ref{fig:add_experiments}. Results have been normalized by the average performance of
Mean imputation for better display effects.

Results show that IGRM yields 12.93\%, 16.93\% and 23.67\% lower mean of MAE than the second-best baselines in MCAR, MAR and MNAR mechanisms respectively. 
In addition, IGRM outperforms all baselines in all datasets in MCAR mechanisms and it outperforms baselines except KNN and MICE in Ai4i dataset in MAR mechanism.

% \begin{table}[htb]
%  \centering
%   \caption{Properties of additional datasets used in experiments, Disc. short for Discrete and Cont. short for continuous.}
%     \begin{tabular}{lrrr}
%     \toprule
%     \textbf{Dataset}  & \textbf{Samples \#} & \textbf{Disc. F. \#} & \textbf{Cont. F. \#} \\
%     \midrule
%     Blood & 748 & 0 & 4 \\
%     Steel & 1941 & 0 & 33 \\
%     Phoneme & 5404 & 0 & 5 \\
%     Abalone & 4177 & 1 & 7 \\
%     Energy & 768 & 0 & 8 \\
%     Cmc & 1473 & 8 & 1 \\
%     German & 1000 & 13 & 7 \\
%     Ai4i & 10000 & 7 & 5 \\
%     \bottomrule
%     \end{tabular}
%   \label{tab:datasets_appendix}
%   \vspace{-0.1in}
% \end{table}%

\begin{table*}[htb]
    \centering
    \begin{tabular}{lrrrrrrrr}
    \toprule
    \textbf{Dataset} & Blood & Steel & Phoneme & Abalone & Energy & Cmc & German & Ai4i \\
    \midrule
    \textbf{Samples \#} & 748 & 1941 & 5404 & 4177 & 768 & 1473 & 1000 & 10000 \\
    \textbf{Disc. F. \#} & 0 & 0 & 0 & 1 & 0 & 8 & 13 & 7 \\
    \textbf{Cont. F. \#} & 4 & 33 & 5 & 7 & 8 & 1 & 7 & 5 \\
    \bottomrule
    \end{tabular}
    \caption{Properties of additional datasets used in experiments, Disc. short for Discrete and Cont. short for continuous.}
    \label{tab:datasets_appendix}
\end{table*}

\begin{figure*}[htb]
    \centering
    \includegraphics[width=1.0\textwidth]{}
    \caption{Imputation methods on 8 datasets from the UCI repository in 30\% missing in MCAR(top), MAR(middle), MNAR(bottom) mechanisms. The result is normalized by the average performance of Mean imputation.}
    \label{fig:add_experiments}
    % \vspace{-0.1in}
\end{figure*}

\subsection{Initialization Method Details}
In this section, we provide details about the initialization of IGRM-rule.
\subsubsection{IGRM-rule} is initialized by association rules, since we consider that two samples with the same rules are similar in feature sub-spaces.
Since majority of our datasets have mixed data types, before mining rules, the continuous features of $\mathbf{D}$ is discretized by the cluster binning technique which is determined by Davies-Bouldin index\cite{davies1979cluster}, resulted in $\hat{\mathbf{D}}$.
In this work, we adopt FP-growth\cite{han2000mining} to mine the frequent itemsets in observed values, and set the default minimum support and confidence as 0.1 and 0.6 respectively while in Housing dataset the minimum confidence is 0.7 and in E-commerce dataset the minimum confidence is 0.5 to obtain association rules.
An association rule can be formed as $\mathcal{R}:\mathbf{A}\Rightarrow\mathbf{B}$, where $\mathbf{A}$ is antecedent and $\mathbf{B}$ is consequent, $\mathbf{A}\cap \mathbf{B}=\varnothing$.
The items in $\mathbf{A}$ and $\mathbf{B}$ are denoted as $a_1,a_2,...,a_n$ and $b$.

Candidate node set $\mathbf{C}$ contains sample nodes whom both $\mathbf{A}$ and $\mathbf{B}$ exist in, $\mathbf{C}=\{u_{i}|(\mathbf{A}\cup \mathbf{B})\subseteq \{\mathbf{D}_{ij}|\mathbf{N}_{ij}=1,j=1,...,m\}\}$. For each time, we sample and connect a pair of nodes without replacement from $\mathbf{C}$, repeats this work until $\mathbf{C}$ is empty.

\clearpage
